# Supplementary material for: Clifford Quantum Cellular Automata: Trivial group in 2D and Witt group in 3D
Source: arXiv:1907.02075 source file (2022-05-19)
Supplement: Supplementary file 1 [file clifqca-v2-supp-output.pdf]

18 October 2019, Jeongwan Haah

# Tools

All routines here do not depend on the characteristic of the base field. So they are applicable for stabilizer codes on qudits of prime dimensions. The naming policy for functions is such that the first letter is in lower case in order to distinguish it from *Mathematica*'s own functions. The scripts in Tools section were contained in [Haah, arXiv:1310.4507] which is based on [Haah, arXiv:1204.1063].

## Variables of Laurent polynomial ring:

In[1]:=
```
Protect[x, y, z, w];
```

In[2]:=
```
translationVariables = {x, y, z, w};
```

## display( mat )

In[3]:=
```
insertIndex[mat_] := Block[{qind, cind},
   qind = Table[i, {i, 1, First@Dimensions[mat] / 2}];
   cind = Table[i, {i, 1, Last@Dimensions[mat]}];
   Transpose[Join[{Join[{"\\"}, qind, qind]}, Transpose[Join[{cind}, mat]]]]
  ]
```

In[4]:=
```
show[mat_] := MatrixForm@insertIndex[mat]
display[mat_] := MatrixForm[insertIndex[Expand[mat]]]
display2[mat_] := MatrixForm[insertIndex[Expand[PolynomialMod[mat, 2]]]]
 (*for qubit-stabilizer codes*)
```

In[7]:=
```
pmod2[x_] := PolynomialMod[x, 2]
```

## antipode(f): an involutive automorphism of Laurent polynomial ring
## dagger = antipode followed by transpose
## symprod[v, w] = symplectic product = dagger[v].$\lambda$.w

In[8]:=
```
antipode[f_] := (f /. {x → 1/x, y → 1/y, z → 1/z, w → 1/w})
```

In[9]:=
```
dagger[m_] := Transpose@antipode[m]
```

In[10]:=
```
symplecticMatrix[n_] := KroneckerProduct[{{0, 1}, {-1, 0}}, IdentityMatrix[n]]
symprod[v_, w_] := Expand[dagger[v].symplecticMatrix[Length[w] / 2].w]
```

### coarseGrain(mat, {var, n})

In[12]:=
```
expandEntry[poly_, x_, n_] := Module[{f, p, c, xp, col, monos, exps, gen},
  f[i_, j_] := If[i - 1 == j, 1, If[i - 1 + n == j, x, 0]];
  gen = Table[f[i, j], {i, 1, n}, {j, 1, n}];
  p = Expand[poly];
  If[p === 0,
   (*return zero matrix if the input is zero*)
   Table[0, {n}, {n}],
   (*Else, compute properly*)
   col = Collect[p, x];
   monos = If[Head[col] === Plus, Apply[List, col], {col}];
   exps = Map[Exponent[#, x] &, monos];
   c = Power[x, -exps] * monos;
   xp = Map[MatrixPower[gen, #] &, exps];
   Expand[c.xp]
   (*end-if*)]
 ]
```

In[13]:=
```
coarseGrain[mat_, {x_, n_}] :=
 Apply[Join, Table[
   Join[Table[
     Flatten[
      Map[expandEntry[#, x, n][[nn]] &, mat[[row]]]
     ], {nn, n}]
   ], {row, Length[mat]}]
 ]
```

# Remark on symprod

The most important function that is used below but is not a part of Mathematica, is symprod. It takes two inputs v1 v2, where the first one v1 is sent through the antipode that inverts all the translation variables x,y,z, and then computes the “symplectic” product v1^dagger. lambda. v2. Here lambda is the standard symplectic matrix with -1,0,1 entries. The output captures all the relative positions of the two Pauli operators corresponding to v1 and v2 such that they are noncommuting. The positional information is encoded in the exponents, and the phase of the commutation relation in the coefficients.

The name “symplectic” should be read with some care. Strictly speaking, the product is not symplectic as the product of v with itself is not zero in general. Perhaps it is more appropriate to use a terminology “antihermitian form” but this has disadvantage that it may be confused with antihermitian operators on a complex inner product space (Hilbert space). We stick with “symplectic product” since, at least, it becomes symplectic when restricted to F_p without any variables. We speak of “antihermitian form” on a module over Laurent polynomial rings, obtained by taking the symplectic product among the

generators.

# Construction by condensation for a system of odd prime dimensional qudits

## Stabilizer map of the toric code

In[14]:= sigmaToric = $\begin{pmatrix} y-1 & 0 \\ -x+1 & 0 \\ 0 & \frac{1}{x}-1 \\ 0 & \frac{1}{y}-1 \end{pmatrix}$;

```
In[15]:= symprod[sigmaToric, sigmaToric]
Out[15]= {{0, 0}, {0, 0}}
```

This says that the terms of the toric code are commuting with each other.

## Coupling layers

The following displays hopping terms for the bound state of a particle in a layer with its time reversal conjugate in the upper layer, corrected so that they commute with each other.

In[16]:= sigmaQCA = $\begin{pmatrix} f z + f & 0 \\ 0 & f z + f \\ 0 & z y - y \\ -z x + x & 0 \end{pmatrix}$ + sigmaToric.$\begin{pmatrix} f + f x z & -f y - f z \\ 0 & 0 \end{pmatrix}$;

```
symprod[sigmaQCA, sigmaQCA]
sigmaQCA // Expand // MatrixForm
Out[17]= {{0, 0}, {0, 0}}
```

Out[18]//MatrixForm=

$$\begin{pmatrix} f y + f z - f x z + f x y z & f y - f y^2 + f z - f y z \\ f - f x + f x z - f x^2 z & f - f y + f x y + f x z \\ 0 & -y + y z \\ x - x z & 0 \end{pmatrix}$$

## Ground state nondegeneracy of the bulk Hamiltonian

```
In[19]:= minors = Minors[sigmaQCA, 2] // Flatten // Simplify
```

Out[19]= $\{f^2 x y (1+z)^2, f y (-1+z) (y+z-x z+x y z), -f x (-1+y) (-1+z) (y+z), -(-1+x) y (-1+z) (f+f x z), f x (-1+z) (1+(-1+x) y+x z), x y (-1+z)^2\}$

The first and the last factors generate 4 z, which is a unit. Therefore, the determinantal ideal is unit, when the field has characteristic different from 2. This implies that the commuting Pauli Hamiltonian

(stabilizer code Hamiltonian) defined by sigmaQCA has nondegenerate ground state on any 3-torus.

# QCA and antihermitian form (over odd prime)

In[20]:= qca =

$$\begin{pmatrix} \frac{1}{4}-\frac{xz}{4}+\frac{z}{4y}+\frac{xyz}{4} & \frac{z}{4}+\frac{yz}{4}-\frac{xyz}{4}+\frac{1}{4}xy^2z & fy+fz-fxz+fxyz & fy-fy^2+fz-fyz \\ \frac{x}{4}+\frac{1}{4y}-\frac{x^2z}{4}+\frac{xz}{4y} & \frac{1}{4}+\frac{xz}{4}+\frac{xyz}{4}-\frac{1}{4}x^2yz & f-fx+fxz-fx^2z & f-fy+fxy+fxz \\ -\frac{1}{4f}-\frac{y}{4f}+\frac{xz}{4f}-\frac{xyz}{4f} & -\frac{y}{4fx}+\frac{xyz}{4f} & 0 & -y+yz \\ \frac{xy}{4f}-\frac{xz}{4fy} & -\frac{1}{4f}+\frac{y}{4f}-\frac{xz}{4f}-\frac{xyz}{4f} & x-xz & 0 \end{pmatrix};$$

```
In[21]:= qca[[ ;; , {3, 4}]] == sigmaQCA // Simplify
```

Out[21]= True

```
In[22]:= symprod[qca, qca] // MatrixForm
```

Out[22]//MatrixForm=

$$\begin{pmatrix} 0 & 0 & 1 & 0 \\ 0 & 0 & 0 & 1 \\ -1 & 0 & 0 & 0 \\ 0 & -1 & 0 & 0 \end{pmatrix}$$

We have to find a minimal generating set for the span of coefficient of z in qca. It suffices to take the coefficient of z in sigmaQCA, because, as we see in the following line, the coefficient of z in the first two columns of qca is redundant.

```
In[23]:= B$generator = Coefficient[sigmaQCA, z];
% // MatrixForm
```

Coefficient[qca[[ ;; , {1, 2}]], z] == $\frac{1}{4f}$ B$generator. $\begin{pmatrix} \frac{1}{y} & 1+y \\ \frac{x}{y}-x & x \end{pmatrix}$ // Expand

Out[24]//MatrixForm=

$$\begin{pmatrix} f-fx+fxy & -f(-1+y) \\ f(1-x)x & fx \\ 0 & y \\ -x & 0 \end{pmatrix}$$

Out[25]= True

Thus, the following is the antihermitian form of the boundary algebra.

In[26]:= B$generator. $\begin{pmatrix} 1 & 0 \\ 0 & x \end{pmatrix}$ // Expand;

symprod[%, %] // MatrixForm

Out[27]//MatrixForm=

$$\begin{pmatrix} \frac{f}{x}-fx & f+fx-fy+fxy \\ -f-\frac{f}{x}+\frac{f}{y}-\frac{f}{xy} & -\frac{f}{y}+fy \end{pmatrix}$$

The determinant is a square of the ground field as promised.

In[28]:=
```
% // Det
```
Out[28]= $4\,f^2$

# Surface topological order (over odd prime)

bulk occupies z <= 0 and the surface lies at z = 0

## Introducing surface terms

In[29]:=
$$\text{surfaceTerms} = \begin{pmatrix} f\,x\,(-1+y)\,y \\ -f\,(-1+x)\,x\,y \\ (-1+x)\,y \\ x\,(-1+y) \end{pmatrix};$$

In[30]:=
```
symprod[surfaceTerms, surfaceTerms]
```
Out[30]=
```
{{0}}
```

The surface terms commute with each other.

## Commuting with the bulk terms

In[31]:=
```
bulkTermsOnSurface = Coefficient[sigmaQCA, z];
bulkTermsOnSurface // display
```
Out[32]//MatrixForm=

$$\begin{pmatrix} \backslash & 1 & 2 \\ 1 & f - f\,x + f\,x\,y & f - f\,y \\ 2 & f\,x - f\,x^2 & f\,x \\ 1 & 0 & y \\ 2 & -x & 0 \end{pmatrix}$$

In[33]:=
```
symprod[surfaceTerms, bulkTermsOnSurface]
```
Out[33]=
```
{{0, 0}}
```

The surface terms commute with all the bulk terms.

## Local topological order

We compute the rank and codimension of the determinantal ideals to apply Buchsbaum-Eisenbud criterion to check that any operator at the surface that commutes with all bulk and surface terms is a product of surface terms.

In[34]:=
```
combined = Transpose@Join[Transpose@surfaceTerms , Transpose@bulkTermsOnSurface];
combined // display
```

Out[35]//MatrixForm=

$$\begin{pmatrix} \backslash & 1 & 2 & 3 \\ 1 & -f x y + f x y^2 & f - f x + f x y & f - f y \\ 2 & f x y - f x^2 y & f x - f x^2 & f x \\ 1 & -y + x y & 0 & y \\ 2 & -x + x y & -x & 0 \end{pmatrix}$$

In[36]:=
```
Minors[combined, 3] // Simplify
```

Out[36]= $\{\{2 f^2 (-1+x) x y^2\}, \{2 f^2 x^2 (-1+y) y\}, \{2 f x^2 (-1+y) y^2\}, \{-2 f (-1+x) x^2 y^2\}\}$

The combined has rank 3 and the determinantal ideal is (x-1,y-1) of depth 2. (Recall that we're over the Laurent polynomial ring, so any monomial is a unit.)

In[37]:=
```
Minors[surfaceTerms, 1] // Simplify
```

Out[37]= $\{\{f x (-1+y) y\}, \{-f (-1+x) x y\}, \{(-1+x) y\}, \{x (-1+y)\}\}$

The surfaceTerms has rank 1 and the determinantal ideal is (y-1,x-1) of depth 2.

Therefore, the Buchsbaum-Eisenbud criterion is met, and the surfaceTerms generates a maximal commutative subalgebra in the commutant of the bulkTermsOnSurface.

## Hopping operators for surface anyons

In[38]:= $hx = \frac{x y}{2} \begin{pmatrix} y \\ 1 - x \\ 0 \\ x / f \end{pmatrix}; hy = \frac{x y}{2} \begin{pmatrix} y - y^2 \\ x y - y + 1 \\ -y / f \\ 0 \end{pmatrix};$

The commutation relation of these hopping operators is the negative of the antihermitian form above (up to a congruence by monomials). This is consistent since the hopping operators generate the commutant of the bulk operators (B$generators).

In[39]:=
```
Transpose@Join[Transpose@hx, Transpose@hy];
symprod[%, %] // MatrixForm
```

Out[40]//MatrixForm=

$$\begin{pmatrix} -\frac{1}{4 f x} + \frac{x}{4 f} & -\frac{1}{4 f} - \frac{1}{4 f x} - \frac{y}{4 f} + \frac{y}{4 f x} \\ \frac{1}{4 f} + \frac{x}{4 f} + \frac{1}{4 f y} - \frac{x}{4 f y} & \frac{1}{4 f y} - \frac{y}{4 f} \end{pmatrix}$$

## Checking commutation relations

In[41]:=
```
symprod[surfaceTerms, hx]
symprod[surfaceTerms, hy]
symprod[bulkTermsOnSurface, hx]
symprod[bulkTermsOnSurface, hy]
symprod[Coefficient[qca, z], hx]
symprod[Coefficient[qca, z], hy]
```

Out[41]= {{-1 + x}}

Out[42]= {{-1 + y}}

Out[43]= {{0}, {0}}

Out[44]= {{0}, {0}}

Out[45]= {{0}, {0}, {0}, {0}}

Out[46]= {{0}, {0}, {0}, {0}}

hx commutes with all but two surface terms. The noncommuting surface terms acquires phase factors of opposite exponents upon conjugation by hx, and are separated by distance 1 along x-axis. In other words, hx annihilates a particle represented by a flipped surface term at (0,0), and creates a particle at (1,0). hy does the same along y-axis. Both hx and hy commute with all the bulk terms. They even commute with elements of the local flipper which are contained in the lower half space z <= 0, and generate the commutant of the algebra of all elements of the separator and of the local flipper which are supported on the half space z <=0, as checked by the following Buchsbaum-Eisenbud criterion.

In[47]:=
```
Minors[Coefficient[qca, z], 3]
GroebnerBasis[Minors[Coefficient[qca, z], 2], {x, y}]
Minors[Join[Transpose[hx], Transpose[hy]], 2]
GroebnerBasis[%, {x, y}]
```

Out[47]= {{0, 0, 0, 0}, {0, 0, 0, 0}, {0, 0, 0, 0}, {0, 0, 0, 0}}

Out[48]= {1}

Out[49]= $\left\{\left\{\frac{x^3 y^3}{4}, -\frac{x^2 y^4}{4 f}, -\frac{x^3 y^3}{4 f}+\frac{x^3 y^4}{4 f}, -\frac{x^2 y^3}{4 f}+\frac{x^3 y^3}{4 f}, -\frac{x^3 y^2 (1-y+x y)}{4 f}, \frac{x^3 y^3}{4 f^2}\right\}\right\}$

Out[50]= $\{x^2 y^3, x^3 y^2\}$

The following line shows that the loop of the hopping operators is the surface term.

In[51]:= $(hx\ (y-1) - (x-1)\ hy)\ \frac{2 f}{x y}$ == surfaceTerms // Simplify

Out[51]= True

## Topological spin of excitations

In[52]:=
```
constantTerm[poly_] := Select[Apply[List, poly], Simplify[# == antipode[#]] &]
```

In[53]:=
```
theta[stringLength_] := Block[{},
  t1 = Sum[x^m, {m, 0, stringLength}] hx;
  t2 = Sum[y^m, {m, 0, stringLength}] hy;
  t3 = Sum[x^m, {m, 0, -stringLength, -1}] (-hx / x);
  symprod[t1, -t2] + symprod[t1, t3] + symprod[-t2, t3]
 ]
```

The "constant" term is the exponent of the phase factor in the commutation relation t1 t2^dagger t3 = $e^{i\theta}$ t3 t2^dagger t1.

In[54]:=
```
theta[0]
theta[0] // First // First // constantTerm
theta[3] // First // First // constantTerm
theta[10] // First // First // constantTerm
```

Out[54]= $\left\{\left\{\frac{1}{4\,f}+\frac{1}{4\,f\,x^2}+\frac{1}{2\,f\,x}-\frac{1}{4\,f\,y}+\frac{1}{4\,f\,x\,y}+\frac{y}{4\,f}-\frac{y}{4\,f\,x}\right\}\right\}$

Out[55]= $\left\{\frac{1}{4\,f}\right\}$

Out[56]= $\left\{\frac{1}{4\,f}\right\}$

Out[57]= $\left\{\frac{1}{4\,f}\right\}$

We do not have to check a larger stringLength since the long hopping operators t1,t2,t3 are of width 2 that is much smaller than 10 and we know theta cannot depend on tensor components that are far from the intersection at the origin.

# With Qubits (p=2)

The coupled layer construction with qubits is more complicated than with odd prime dimensional qudits. This is due to the fact that a single copy of the toric code does not have any modular proper subtheory, and we have to bring two copies of the toric code to have an interesting decomposition. Except for this complication, the calculation at a conceptual level is identical as above. A nontrivial result from the consideration of boundary algebras below is that the two Hamiltonians, one by Walker and Wang tailored to 3-fermion theory by Burnell, Chen, Fidkowski, and Vishwanath (arXiv:1302.7072), and the other constructed here following Chong and Senthil (arXiv.1302.6234)’s prescription, are equivalent up to a Clifford circuit. It also shows that the two QCA that disentangle the respective ground states, are equivalent up to Clifford circuits and shifts.

In[58]:=

$$p1 = \begin{pmatrix} 0 \\ 0 \\ 0 \\ 0 \\ 1 + y \\ 1 + x \\ 0 \\ 0 \end{pmatrix};$$

$$p2 = \begin{pmatrix} 0 \\ 0 \\ 0 \\ 0 \\ 0 \\ 0 \\ 1 + y \\ 1 + x \end{pmatrix};$$

$$s1 = \begin{pmatrix} 1 + x^{-1} \\ 1 + y^{-1} \\ 0 \\ 0 \\ 0 \\ 0 \\ 0 \\ 0 \end{pmatrix};$$

$$s2 = \begin{pmatrix} 0 \\ 0 \\ 1 + x^{-1} \\ 1 + y^{-1} \\ 0 \\ 0 \\ 0 \\ 0 \end{pmatrix};$$ (*The plaquette and star operators*)

In[59]:=

$$e1h = \begin{pmatrix} 1 \\ 0 \\ 0 \\ 0 \end{pmatrix}; e1v = \begin{pmatrix} 0 \\ 1 \\ 0 \\ 0 \end{pmatrix}; e2h = \begin{pmatrix} 0 \\ 0 \\ 1 \\ 0 \end{pmatrix}; e2v = \begin{pmatrix} 0 \\ 0 \\ 0 \\ 1 \end{pmatrix};$$ (*Basis vectors for edges*)

In[60]:=
```
hy$lower = KroneckerProduct[{{x^-1}, {0}}, e1h + e2h] +
    KroneckerProduct[{{0}, {y^-1}}, e1v] + (x^-1 + x^-1 y^-1) (p1 + p2) + s2 + y^-1 s1;
hy$upper = KroneckerProduct[{{x^-1}, {0}}, e1h + e2h] + KroneckerProduct[{{0}, {y^-1}}, e2v] +
    (x^-1 + x^-1 y^-1) (p1 + p2) + s2 + y^-1 s1;
hy$p2 = hy$lower + z hy$upper; (*The hopping operator for eps1-
 e2 pairs along x- and y-direction.*)
hx$lower = KroneckerProduct[{{0}, {1}}, e1h + e2h] +
    KroneckerProduct[{{x y^-1}, {0}}, e1v] + (s1 + s2) (1 + x) + p1 y^-1 + p2 x y^-1;
hx$upper = KroneckerProduct[{{0}, {1}}, e1h + e2h] + KroneckerProduct[{{x y^-1}, {0}}, e2v] +
    (s1 + s2) (1 + x) + p1 y^-1 + p2 x y^-1;
hx$p2 = hx$lower + z hx$upper;
```

In[66]:=
```
ty$lower = KroneckerProduct[{{0}, {1}}, e1v + e2v] +
    KroneckerProduct[{{1}, {0}}, e1h] + (1 + y) (s1 + s2) + p2 + y^-1 p1;
ty$upper = KroneckerProduct[{{0}, {1}}, e1v + e2v] + KroneckerProduct[{{1}, {0}}, e2h] +
    (1 + y) (s1 + s2) + p2 + y^-1 p1;
ty$p2 = ty$lower + z ty$upper; (*The hopping operator for eps1-
 m2 pairs along x- and y-direction.*)
tx$lower = KroneckerProduct[{{1}, {0}}, e1v + e2v] +
    KroneckerProduct[{{0}, {1}}, e1h] + (p1 + p2) (1 + x^-1) + s1 + s2 x;
tx$upper = KroneckerProduct[{{1}, {0}}, e1v + e2v] + KroneckerProduct[{{0}, {1}}, e2h] +
    (p1 + p2) (1 + x^-1) + s1 + s2 x;
tx$p2 = tx$lower + z tx$upper;
```

In[72]:=
```
separator = Transpose@Join[y^-1 Transpose@tx$p2,
      y^-1 Transpose@ty$p2, Transpose@hx$p2, x Transpose@hy$p2] // pmod2;
symprod[separator, separator] // pmod2
```

Out[73]=
```
{{0, 0, 0, 0}, {0, 0, 0, 0}, {0, 0, 0, 0}, {0, 0, 0, 0}}
```

This separator gives an exactly solvable model of three-fermion Walker-Wang model, following a prescription in [Chong, Senthil, arXiv.1302.6234].

In[74]:=
```
varxyz = {x, xi, y, yi, z, zi};
invxyz = {x xi - 1, y yi - 1, z zi - 1};
inv = {xi → 1 / x, yi → 1 / y, zi → 1 / z};
```

In[77]:=
```
Dimensions[separator]
```

Out[77]= {8, 4}

In[78]:=
```
GroebnerBasis[{Minors[separator, 4], invxyz}, varxyz, Modulus → 2]
```

Out[78]= {1}

Therefore, separator is a separator.

In[79]:=
```
B$generator$p2 = Coefficient[separator // Expand, z];
```

In[80]:=
```
symprod[B$generator$p2, B$generator$p2] // pmod2 // Expand // MatrixForm
```

Out[80]//MatrixForm=

$$\begin{pmatrix} \frac{1}{x}+x & 1 & 0 & 1+x+y+xy \\ 1 & \frac{1}{y}+y & 1+x+y+xy & 0 \\ 0 & 1+\frac{1}{x}+\frac{1}{y}+\frac{1}{xy} & \frac{1}{x}+x & 1 \\ 1+\frac{1}{x}+\frac{1}{y}+\frac{1}{xy} & 0 & 1 & \frac{1}{y}+y \end{pmatrix}$$

This is an antihermitian form induced from a disentangling QCA of the coupled layer model.

In[81]:=
```
Det[%] // pmod2
```

Out[81]= 1

## Comparison to the previous QCA over qubits

In [Burnell, Chen, Fidkowski, Vishwanath, arXiv:1302.7072] a Hamiltonian with three-fermion topological order at the surface was presented, which happens to be a commuting Pauli Hamiltonian, whose stabilizer map is the following.

In[82]:= sigma3FWW =

$$\begin{pmatrix} 1+x^{-1} & 0 & 0 & 0 & x^{-1}+yz & 0 & 0 & yz \\ 1+y^{-1} & 0 & 0 & y^{-1}+xz & 0 & 0 & xz & 0 \\ 1+z^{-1} & 0 & z^{-1}+xy & 0 & 0 & xy & 0 & 0 \\ 0 & 1+x^{-1} & 0 & 0 & x^{-1} & 0 & 0 & x^{-1}+yz \\ 0 & 1+y^{-1} & 0 & y^{-1} & 0 & 0 & y^{-1}+xz & 0 \\ 0 & 1+z^{-1} & z^{-1} & 0 & 0 & z^{-1}+xy & 0 & 0 \\ 0 & 0 & 1+y & 1+z & 0 & 0 & 0 & 0 \\ 0 & 0 & 1+x & 0 & 1+z & 0 & 0 & 0 \\ 0 & 0 & 0 & 1+x & 1+y & 0 & 0 & 0 \\ 0 & 0 & 0 & 0 & 0 & 1+y & 1+z & 0 \\ 0 & 0 & 0 & 0 & 0 & 1+x & 0 & 1+z \\ 0 & 0 & 0 & 0 & 0 & 0 & 1+x & 1+y \end{pmatrix};$$

We find a Clifford circuit followed by a shift, to somehow simplify this stabilizer map.

In[83]:= **cliffordCircuitShift =**

$$\left(\begin{array}{cc}
\frac{1}{y\,z} & 0 \\
0 & \frac{1}{x\,z}\cdots \\
0 & 0 \\
1+y+x\,y+x\,y^2+\frac{1}{z}+\frac{y}{z}+x\,y\,z+x\,y^2\,z & \frac{1}{x}+\frac{y}{x}+y^2+\frac{1}{x}\cdots \\
x^2+\frac{1}{y}+\frac{x}{y}+\frac{1}{y\,z}+\frac{x}{y\,z}+x\,z+x^2\,z+\frac{x\,z}{y} & 1+\frac{1}{y}+\frac{1}{x\,y}+x\,y+\frac{1}{y\,z}+\cdots \\
1+\frac{1}{z} & \frac{1}{x}+\cdots \\
0 & 1+\cdots \\
1+\frac{1}{z} & 0 \\
x+x\,y & y+\cdots \\
x+y+x^2\,y+x^2\,y^2+\frac{x}{z}+\frac{x\,y}{z}+z+x\,z+y\,z+x^2\,y\,z+x^2\,y^2\,z & 1+\frac{y}{x}+x\,y^2+\frac{1}{z}+\frac{y}{z}+\cdots \\
1+x\,y+x^2\,y+\frac{1}{z}+\frac{x}{z}+x\,z+x\,y\,z+x^2\,y\,z & 1+\frac{1}{x}+y+x\,y+\frac{1}{z}\cdots \\
x\,z+x\,y\,z & y\,z+\cdots
\end{array}\right.$$

It is left to the readers to verify that the above matrix is a product of elementary symplectic transformations.

In[84]:= **rearrangement =**

$$\left(\begin{array}{cccccccc}
x\,y+\frac{1}{x\,y\,z^2}+\frac{1}{z} & 1+x\,y\,z & 0 & 0 & 0 & 1 & z+x\,y\,z^2 & y\,z+x\,y^2\,z^2 \\
0 & 1 & 0 & 0 & 0 & 0 & 0 & 0 \\
1+\frac{1}{x\,y\,z^2}+\frac{1}{z}+\frac{1}{x\,y\,z} & 1+z & 1 & 0 & 0 & \frac{1}{x\,y} & \frac{1}{x\,y}+z+\frac{z}{x\,y}+z^2 & \frac{1}{x}+\frac{z}{x}+y\,z+y\,z^2 \\
\frac{1}{x\,z^2}+\frac{1}{x\,y\,z^2}+\frac{1}{z}+\frac{y}{z} & 1+y & 0 & 1 & 0 & \frac{1}{x\,z}+\frac{1}{x\,y\,z} & \frac{1}{x}+\frac{1}{x\,y}+\frac{1}{x\,y\,z}+z+y\,z & \frac{1}{x}+\frac{y}{x}+y\,z+y^2\,z \\
\frac{1}{y\,z^2}+\frac{1}{x\,y\,z^2}+\frac{1}{z}+\frac{x}{z} & 1+x & 0 & 0 & 1 & \frac{1}{y\,z}+\frac{1}{x\,y\,z} & \frac{1}{y}+\frac{1}{x\,y}+z+x\,z & 1+\frac{1}{x}+\frac{1}{x\,y\,z}+y\,z+x\,y\,z \\
\frac{1}{x\,y\,z^2}+\frac{1}{x\,y\,z} & 0 & 0 & 0 & 0 & 1 & 0 & 0 \\
\frac{1}{x\,z^2}+\frac{1}{x\,y\,z^2} & 0 & 0 & 0 & 0 & 0 & 1 & 0 \\
\frac{1}{y\,z^2}+\frac{1}{x\,y\,z^2} & 0 & 0 & 0 & 0 & 0 & 0 & 1
\end{array}\right);$$

In[85]:=
```
deformed$3FWW = cliffordCircuitShift.sigma3FWW.rearrangement // pmod2;
% // display2
```

Out[86]//MatrixForm=

| \ | 1 | 2 | 3 | 4 | 5 | 6 | 7 | 8 |
|---|---|---|---|---|---|---|---|---|
| 1 | 0 | 0 | 0 | 0 | 1 | 0 | 0 | 0 |
| 2 | 0 | 0 | 0 | 1 | 0 | 0 | 0 | 0 |
| 3 | 0 | 0 | $x y$ | 0 | 0 | 0 | 0 | 0 |
| 4 | 0 | 0 | 0 | 0 | 0 | 0 | $1 + z + x y z + x y z^2$ | 0 |
| 5 | 0 | 0 | 0 | 0 | 0 | 0 | $1 + x + \frac{1}{y} + \frac{x}{y} + x^2 z + x y z + x^2 y z$ | $y + \frac{z}{y} + x y^2 z + x z^2$ |
| 6 | 0 | 0 | 0 | 0 | 0 | 1 | 0 | 0 |
| 1 | 0 | 0 | 0 | 0 | 0 | 0 | 0 | 0 |
| 2 | 0 | 0 | 0 | 0 | 0 | 0 | 0 | 0 |
| 3 | 0 | 0 | 0 | 0 | 0 | 0 | 0 | 0 |
| 4 | 0 | 0 | 0 | 0 | 0 | 0 | $x + \frac{z}{x} + x^2 y z + y z^2$ | $z + \frac{z}{x} + \frac{y z}{x} + y z^2 + x y z^2 + y^2 z^2 + x y^2 z^2$ |
| 5 | 0 | 0 | 0 | 0 | 0 | 0 | 0 | $1 + z + x y z + x y z^2$ |
| 6 | 0 | 0 | 0 | 0 | 0 | 0 | 0 | 0 |

We obtain a separator that is Clifford-circuit equivalent to the three-fermion Walker-Wang model.

In[87]:=
```
s9 = deformed$3FWW[[{4, 5, 10, 11}, {7, 8}]];
display2[s9]
```

Out[88]//MatrixForm=

| \ | 1 | 2 |
|---|---|---|
| 1 | $1 + z + x y z + x y z^2$ | 0 |
| 2 | $1 + x + \frac{1}{y} + \frac{x}{y} + x^2 z + x y z + x^2 y z$ | $y + \frac{z}{y} + x y^2 z + x z^2$ |
| 1 | $x + \frac{z}{x} + x^2 y z + y z^2$ | $z + \frac{z}{x} + \frac{y z}{x} + y z^2 + x y z^2 + y^2 z^2 + x y^2 z^2$ |
| 2 | 0 | $1 + z + x y z + x y z^2$ |

According to the definition in the main text, we should take a smaller translation group along z-direction.

In[89]:=
```
B$generator$p2 = Coefficient[s9 ~ coarseGrain ~ {z, 2}, z];
symprod[B$generator$p2, B$generator$p2] // Det // pmod2
```

Out[90]= 1

Since the determinant of the commutation relation among the top-operators of the separator is nonzero, there is no need to look at the flipper (or a full QCA) to find an antihermitian form; the symprod we just computed is a legitimate antihermitian form. Next, we apply some column operation to the antihermitian form

In[91]:=
```
rearr1$p2 = {{(1 + x + y + x y)/(x y), (1 + x y + y^2 + x y^3)/(x y^2), 1/(x y), 1/(x y^2)},
   {x + y + x y, (1 + x y + y^2 + x y^3)/y, 1, 1/y}, {0, 1/y, 0, 0}, {0, 1/y, 0, 1/y}};
Det[
 rearr1$p2]
```

Out[92]= $-\frac{1}{x\,y^3}$

In[93]:=
```
B$generator$p2.rearr1$p2;
symprod[%, %] // pmod2 // Expand // MatrixForm
```

Out[94]//MatrixForm=

$$\begin{pmatrix} \frac{1}{x}+x & 1+\frac{1}{x}+x+\frac{1}{y}+\frac{1}{x\,y}+y+x\,y & 0 & 0 \\ 1+\frac{1}{x}+x+\frac{1}{y}+\frac{1}{x\,y}+y+x\,y & \frac{1}{x}+x+\frac{1}{x\,y^2}+x\,y^2 & 0 & 0 \\ 0 & 0 & 0 & 1 \\ 0 & 0 & 1 & 0 \end{pmatrix}$$

To proceed, let us take an even smaller translation group along y-direction.

In[95]:=
```
B$generator$p2$y2 = (B$generator$p2.rearr1$p2) ~coarseGrain~ {y, 2} // pmod2;
symprod[B$generator$p2$y2, B$generator$p2$y2] // pmod2 // Expand // MatrixForm
```

Out[96]//MatrixForm=

$$\begin{pmatrix} \frac{1}{x}+x & 0 & 1+\frac{1}{x}+x & 1+\frac{1}{x}+y+x\,y & 0 & 0 & 0 & 0 \\ 0 & \frac{1}{x}+x & 1+x+\frac{1}{y}+\frac{1}{x\,y} & 1+\frac{1}{x}+x & 0 & 0 & 0 & 0 \\ 1+\frac{1}{x}+x & 1+\frac{1}{x}+y+x\,y & \frac{1}{x}+x+\frac{1}{x\,y}+x\,y & 0 & 0 & 0 & 0 & 0 \\ 1+x+\frac{1}{y}+\frac{1}{x\,y} & 1+\frac{1}{x}+x & 0 & \frac{1}{x}+x+\frac{1}{x\,y}+x\,y & 0 & 0 & 0 & 0 \\ 0 & 0 & 0 & 0 & 0 & 0 & 1 & 0 \\ 0 & 0 & 0 & 0 & 0 & 0 & 0 & 1 \\ 0 & 0 & 0 & 0 & 1 & 0 & 0 & 0 \\ 0 & 0 & 0 & 0 & 0 & 1 & 0 & 0 \end{pmatrix}$$

And then we apply some column operation.

In[97]:=
```
rearr2$p2 = {{1 + x, 1, 1, x, 0, 0, 0, 0}, {x, 1, 1 + x, x, 0, 0, 0, 0},
   {1 + x, 0, 0, x, 0, 0, 0, 0}, {0, 1, 1 + x, 0, 0, 0, 0, 0}, {0, 0, 0, 0, 1, 0, 0, 0},
   {0, 0, 0, 0, 0, 1, 0, 0}, {0, 0, 0, 0, 0, 0, 1, 0}, {0, 0, 0, 0, 0, 0, 0, 1}};
Det[
 rearr2$p2]
```

Out[98]= $-x^2$

In[99]:=
```
B$generator$p2$y2.rearr2$p2;
symprod[%, %] // pmod2 // Expand // MatrixForm
```

Out[100]//MatrixForm=

$$\begin{pmatrix} \frac{1}{x}+x & 1 & 0 & 1+x+y+xy & 0 & 0 & 0 & 0 \\ 1 & \frac{1}{y}+y & 1+x+y+xy & 0 & 0 & 0 & 0 & 0 \\ 0 & 1+\frac{1}{x}+\frac{1}{y}+\frac{1}{xy} & \frac{1}{x}+x & 1 & 0 & 0 & 0 & 0 \\ 1+\frac{1}{x}+\frac{1}{y}+\frac{1}{xy} & 0 & 1 & \frac{1}{y}+y & 0 & 0 & 0 & 0 \\ 0 & 0 & 0 & 0 & 0 & 0 & 1 & 0 \\ 0 & 0 & 0 & 0 & 0 & 0 & 0 & 1 \\ 0 & 0 & 0 & 0 & 1 & 0 & 0 & 0 \\ 0 & 0 & 0 & 0 & 0 & 1 & 0 & 0 \end{pmatrix}$$

This is exactly the same antihermitian matrix that we have seen above, with two extra hyperbolic planes. Therefore, the boundary algebras are isomorphic, and the Hamiltonian of [Burnell,Chen,Fidkowski,Vishwanath, arXiv:1302.7072] is the equivalent up to a Clifford circuit to the Hamiltonian constructed following [Chong, Senthil, arXiv.1302.6234]. The Clifford QCA that disentangle them have to be equivalent.
